# Supplementary material for: Gravitational bremsstrahlung from spinning binaries in the post-Minkowskian expansion
Source: arXiv:2205.15295 source file (2022-08-04)
Supplement: Supplementary file 1 [file SupplementalMaterial.pdf]

# Gravitational bremsstrahlung from spinning binaries in the post-Minkowskian expansion

## Supplemental Material

Massimiliano Maria Riva, Filippo Vernizzi, and Leong Khim Wong
*Université Paris-Saclay, CNRS, CEA, Institut de Physique Théorique, 91191 Gif-sur-Yvette, France*

Here we provide explicit expressions for the components of the radiated four-momentum at leading order in $G$ and up to quadratic order in the spins, the Feynman rules used in the derivation of the stress-energy tensor, the deflections in the bodies' trajectories at first order in $G$, and the integrand of the stress-energy tensor at next-to-leading order in $G$. Computer-readable versions of these expressions are available in the ancillary files attached to the arXiv submission of this paper.

### RADIATED FOUR-MOMENTUM

TABLE I. The component $\mathcal{C}_{u_1}$ of the radiated four-momentum at leading order in $G$. We organize this result in powers of the spins by writing $\mathcal{C}_{u_1} = \mathcal{C}_{u_1}^{(0)} + \Sigma_{A=1}^{2}\mathcal{C}_{u_1}^{s_A} + \Sigma_{A=1}^{2}\Sigma_{B=A}^{2}\mathcal{C}_{u_1}^{s_A s_B} + O(s^3)$, where the superscript $(0)$ denotes the part that is independent of the spins, the superscript $s_1$ denotes the part that is proportional to $s_1$, and so on. The component $\mathcal{C}_{u_2}$ can be obtained directly from $\mathcal{C}_{u_1}$ by interchanging the body labels $1 \leftrightarrow 2$, and note that $\hat{b}$ swaps sign under this interchange.

$\mathcal{C}_{u_1}^{(0)}$

$$\frac{210\gamma^6 - 552\gamma^5 + 339\gamma^4 - 912\gamma^3 + 3148\gamma^2 - 3336\gamma + 1151}{48(\gamma^2-1)^{3/2}} - \frac{35\gamma^4 + 60\gamma^3 - 150\gamma^2 + 76\gamma - 5}{8\sqrt{\gamma^2-1}}\log\left(\frac{1+\gamma}{2}\right) + \frac{70\gamma^7 - 165\gamma^5 + 112\gamma^3 - 33\gamma}{16(\gamma^2-1)^2}\cosh^{-1}\gamma$$

$\mathcal{C}_{u_1}^{s_1}$

$$\frac{(s_1\cdot\hat{l}\,)}{b}\left[\frac{210\gamma^6 - 356\gamma^5 - 111\gamma^4 - 1627\gamma^3 + 5393\gamma^2 - 4741\gamma + 1352}{16(\gamma+1)(\gamma^2-1)} - \frac{105\gamma^4 + 345\gamma^3 - 405\gamma^2 + 147\gamma - 48}{8(\gamma+1)}\log\left(\frac{1+\gamma}{2}\right) + \frac{210\gamma^6 - 405\gamma^4 + 135\gamma^2}{16(\gamma^2-1)^{3/2}}\cosh^{-1}\gamma\right]$$

$\mathcal{C}_{u_1}^{s_2}$

$$\frac{(s_2\cdot\hat{l}\,)}{b}\left[\frac{210\gamma^6 - 279\gamma^5 - 219\gamma^4 - 1350\gamma^3 + 4732\gamma^2 - 4243\gamma + 1245}{16(\gamma+1)(\gamma^2-1)} - \frac{21\gamma^4 + 66\gamma^3 - 84\gamma^2 + 30\gamma - 9}{2(\gamma+1)}\log\left(\frac{1+\gamma}{2}\right) + \frac{42\gamma^6 - 81\gamma^4 + 27\gamma^2}{4(\gamma^2-1)^{3/2}}\cosh^{-1}\gamma\right]$$

$\mathcal{C}_{u_1}^{s_1 s_2}$

$$\begin{aligned}
&\frac{(s_1\cdot u_2)(s_2\cdot u_1)}{b^2}\Bigg[-\frac{1782\gamma^7 + 2217\gamma^6 - 20532\gamma^5 + 10959\gamma^4 + 75198\gamma^3 - 153537\gamma^2 + 115776\gamma - 31287}{64(\gamma+1)^2(\gamma^2-1)^{5/2}} \\
&\qquad + \frac{189\gamma^4 - 531\gamma^3 + 819\gamma^2 - 585\gamma + 144}{4(\gamma+1)(\gamma^2-1)^{3/2}}\log\left(\frac{1+\gamma}{2}\right) - \frac{126\gamma^6 - 243\gamma^4 + 81\gamma^2}{16(\gamma^2-1)^3}\cosh^{-1}\gamma\Bigg] \\
&+ \frac{(s_1\cdot\hat{b})(s_2\cdot\hat{b})}{b^2}\Bigg[-\frac{840\gamma^{10} - 227\gamma^9 - 3696\gamma^8 - 9954\gamma^7 + 44798\gamma^6 - 59952\gamma^5 + 55470\gamma^4 - 20398\gamma^3 - 61950\gamma^2 + 90531\gamma - 35462}{64(\gamma+1)^2(\gamma^2-1)^{5/2}} \\
&\qquad + \frac{42\gamma^7 + 162\gamma^6 - 345\gamma^5 + 27\gamma^4 + 240\gamma^3 - 108\gamma^2 + 63\gamma - 81}{4(\gamma+1)(\gamma^2-1)^{3/2}}\log\left(\frac{1+\gamma}{2}\right) - \frac{168\gamma^7 - 414\gamma^5 + 453\gamma^3 - 315\gamma}{16(\gamma^2-1)^2}\cosh^{-1}\gamma\Bigg] \\
&+ \frac{(s_1\cdot\hat{l}\,)(s_2\cdot\hat{l}\,)}{b^2}\Bigg[\frac{840\gamma^8 - 1907\gamma^7 - 752\gamma^6 - 6741\gamma^5 + 48430\gamma^4 - 91325\gamma^3 + 79596\gamma^2 - 33947\gamma + 5806}{16(\gamma^2-1)^{5/2}} \\
&\qquad - \frac{42\gamma^7 + 162\gamma^6 - 345\gamma^5 + 27\gamma^4 + 195\gamma^3 - 153\gamma^2 + 108\gamma - 36}{(\gamma+1)(\gamma^2-1)^{3/2}}\log\left(\frac{1+\gamma}{2}\right) + \frac{168\gamma^9 - 582\gamma^7 + 687\gamma^5 - 318\gamma^3 + 45\gamma}{4(\gamma^2-1)^3}\cosh^{-1}\gamma\Bigg]
\end{aligned}$$

$\mathcal{C}_{u_1}^{s_1 s_1}$

$$\begin{aligned}
&\frac{(s_1\cdot u_2)^2}{b^2}\Bigg[\frac{1260\gamma^8 + 450\gamma^7 - 5670\gamma^6 + 16530\gamma^5 - 15501\gamma^4 - 30600\gamma^3 + 57822\gamma^2 - 21900\gamma - 2391}{320(\gamma+1)^2(\gamma^2-1)^{5/2}} \\
&\qquad + \frac{315\gamma^4 - 1170\gamma^3 + 1620\gamma^2 - 1062\gamma + 297}{32(\gamma+1)(\gamma^2-1)^{3/2}}\log\left(\frac{1+\gamma}{2}\right) + \frac{90\gamma^3 - 135\gamma}{64(\gamma^2-1)^2}\cosh^{-1}\gamma\Bigg] \\
&+ \frac{(s_1\cdot\hat{b})^2}{b^2}\Bigg[\frac{2520\gamma^8 + 3310\gamma^7 - 1495\gamma^6 - 5070\gamma^5 + 2868\gamma^4 + 7686\gamma^3 - 15315\gamma^2 + 6674\gamma + 24022}{320(\gamma+1)^4\sqrt{\gamma^2-1}} \\
&\qquad - \frac{315\gamma^6 + 1065\gamma^5 + 210\gamma^4 - 1866\gamma^3 - 357\gamma^2 + 801\gamma - 168}{32(\gamma+1)^2\sqrt{\gamma^2-1}}\log\left(\frac{1+\gamma}{2}\right) + \frac{630\gamma^5 - 945\gamma^3}{64(\gamma^2-1)}\cosh^{-1}\gamma\Bigg]
\end{aligned}$$

$$+\frac{(s_1\cdot\hat{l}\,)^2}{b^2}\Bigg[\frac{5670\gamma^6-1180\gamma^5-16935\gamma^4-58250\gamma^3+171298\gamma^2-131850\gamma+38447}{320(\gamma+1)^2\sqrt{\gamma^2-1}}$$

$$-\frac{315\gamma^6+1590\gamma^5-975\gamma^4-636\gamma^3+573\gamma^2-954\gamma+87}{32(\gamma+1)^2\sqrt{\gamma^2-1}}\log\left(\frac{1+\gamma}{2}\right)+\frac{630\gamma^5-855\gamma^3-135\gamma}{64(\gamma^2-1)}\cosh^{-1}\gamma\Bigg]$$

$$+\frac{C_{E_1}(s_1\cdot u_2)^2}{b^2}\Bigg[\frac{1260\gamma^8+450\gamma^7-3645\gamma^6+20580\gamma^5-16086\gamma^4-125580\gamma^3+290877\gamma^2-236490\gamma+70074}{320(\gamma+1)^2(\gamma^2-1)^{5/2}}$$

$$+\frac{315\gamma^4-1170\gamma^3+1620\gamma^2-1206\gamma+297}{32(\gamma+1)(\gamma^2-1)^{3/2}}\log\left(\frac{1+\gamma}{2}\right)+\frac{90\gamma^5-81\gamma^3-81\gamma}{64(\gamma^2-1)^3}\cosh^{-1}\gamma\Bigg]$$

$$+\frac{C_{E_1}(s_1\cdot\hat{b})^2}{b^2}\Bigg[-\frac{4305\gamma^{10}-3500\gamma^9-13415\gamma^8-20740\gamma^7+117647\gamma^6-132330\gamma^5+75309\gamma^4+1280\gamma^3-127504\gamma^2+155290\gamma-56342}{320(\gamma+1)^2(\gamma^2-1)^{5/2}}$$

$$+\frac{525\gamma^7+1530\gamma^6-2385\gamma^5-2220\gamma^4+2643\gamma^3+834\gamma^2-783\gamma-144}{32(\gamma+1)(\gamma^2-1)^{3/2}}\log\left(\frac{1+\gamma}{2}\right)$$

$$-\frac{1050\gamma^9-3675\gamma^7+4632\gamma^5-2655\gamma^3+648\gamma}{64(\gamma^2-1)^3}\cosh^{-1}\gamma\Bigg]$$

$$+\frac{C_{E_1}(s_1\cdot\hat{l}\,)^2}{b^2}\Bigg[\frac{3045\gamma^8-10040\gamma^7+8525\gamma^6-47880\gamma^5+217323\gamma^4-372936\gamma^3+296895\gamma^2-108664\gamma+13732}{320(\gamma^2-1)^{5/2}}$$

$$-\frac{525\gamma^7+1845\gamma^6-3555\gamma^5-915\gamma^4+2607\gamma^3-489\gamma^2+423\gamma-441}{32(\gamma+1)(\gamma^2-1)^{3/2}}\log\left(\frac{1+\gamma}{2}\right)$$

$$+\frac{1050\gamma^9-3765\gamma^7+4803\gamma^5-2655\gamma^3+567\gamma}{64(\gamma^2-1)^3}\cosh^{-1}\gamma\Bigg]$$

$$\mathcal{C}_{u_1}^{s_2s_2}\quad\frac{(s_2\cdot u_1)^2}{b^2}\Bigg[\frac{2520\gamma^9+3150\gamma^8-10125\gamma^7-8925\gamma^6+33999\gamma^5-25761\gamma^4-32463\gamma^3+78777\gamma^2-40491\gamma-681}{640(\gamma+1)^2(\gamma^2-1)^{5/2}}$$

$$-\frac{189\gamma^5+189\gamma^4+1134\gamma^3-2682\gamma^2+1701\gamma-531}{64(\gamma+1)(\gamma^2-1)^{3/2}}\log\left(\frac{1+\gamma}{2}\right)+\frac{378\gamma^5-441\gamma^3-189\gamma}{128(\gamma^2-1)^2}\cosh^{-1}\gamma\Bigg]$$

$$+\frac{(s_2\cdot\hat{b})^2}{b^2}\Bigg[\frac{1890\gamma^{11}+5180\gamma^{10}-12005\gamma^9-10125\gamma^8+10748\gamma^7+4788\gamma^6+28686\gamma^5-20414\gamma^4-4486\gamma^3-5496\gamma^2-24833\gamma+26067}{640(\gamma+1)^2(\gamma^2-1)^{5/2}}$$

$$-\frac{693\gamma^7+1773\gamma^6-1935\gamma^5-3999\gamma^4+2799\gamma^3+1671\gamma^2-1557\gamma+555}{64(\gamma+1)(\gamma^2-1)^{3/2}}\log\left(\frac{1+\gamma}{2}\right)+\frac{1386\gamma^7-3243\gamma^5+1524\gamma^3+333\gamma}{128(\gamma^2-1)^2}\cosh^{-1}\gamma\Bigg]$$

$$+\frac{(s_2\cdot\hat{l}\,)^2}{b^2}\Bigg[\frac{945\gamma^{11}+5915\gamma^{10}-3425\gamma^9-29070\gamma^8-37396\gamma^7+175404\gamma^6-30792\gamma^5-253022\gamma^4+182747\gamma^3+66537\gamma^2-112079\gamma+34236}{320(\gamma+1)^2(\gamma^2-1)^{5/2}}$$

$$-\frac{189\gamma^7+729\gamma^6-1755\gamma^5+393\gamma^4+927\gamma^3-957\gamma^2+639\gamma-165}{32(\gamma+1)(\gamma^2-1)^{3/2}}\log\left(\frac{1+\gamma}{2}\right)+\frac{378\gamma^7-939\gamma^5+552\gamma^3+9\gamma}{64(\gamma^2-1)^2}\cosh^{-1}\gamma\Bigg]$$

$$+\frac{C_{E_2}(s_2\cdot u_1)^2}{b^2}\Bigg[\frac{2520\gamma^9+3150\gamma^8-10125\gamma^7-5565\gamma^6+42159\gamma^5-53841\gamma^4-99183\gamma^3+346377\gamma^2-330891\gamma+108279}{640(\gamma+1)^2(\gamma^2-1)^{5/2}}$$

$$-\frac{189\gamma^5+189\gamma^4+1134\gamma^3-2682\gamma^2+1845\gamma-387}{64(\gamma+1)(\gamma^2-1)^{3/2}}\log\left(\frac{1+\gamma}{2}\right)+\frac{378\gamma^7-819\gamma^5+540\gamma^3-243\gamma}{128(\gamma^2-1)^3}\cosh^{-1}\gamma\Bigg]$$

$$+\frac{C_{E_2}(s_2\cdot\hat{b})^2}{b^2}\Bigg[-\frac{1260\gamma^{11}+8400\gamma^{10}-10245\gamma^9-24035\gamma^8-31168\gamma^7+149252\gamma^6-88626\gamma^5+52014\gamma^4-87204\gamma^3-96364\gamma^2+215983\gamma-89267}{640(\gamma+1)^2(\gamma^2-1)^{5/2}}$$

$$+\frac{987\gamma^7+2787\gamma^6-4065\gamma^5-4113\gamma^4+4593\gamma^3+1305\gamma^2-1515\gamma+21}{64(\gamma+1)(\gamma^2-1)^{3/2}}\log\left(\frac{1+\gamma}{2}\right)$$

$$-\frac{1974\gamma^9-6651\gamma^7+7857\gamma^5-4089\gamma^3+909\gamma}{128(\gamma^2-1)^3}\cosh^{-1}\gamma\Bigg]$$

$$+\frac{C_{E_2}(s_2\cdot\hat{l}\,)^2}{b^2}\Bigg[-\frac{630\gamma^9-3885\gamma^8+5940\gamma^7-335\gamma^6+36456\gamma^5-171341\gamma^4+279868\gamma^3-214293\gamma^2+76466\gamma-9506}{320(\gamma^2-1)^{5/2}}$$

$$-\frac{399\gamma^7+1299\gamma^6-2505\gamma^5-621\gamma^4+1941\gamma^3-495\gamma^2+165\gamma-183}{32(\gamma+1)(\gamma^2-1)^{3/2}}\log\left(\frac{1+\gamma}{2}\right)$$

$$+\frac{798\gamma^9-2727\gamma^7+3249\gamma^5-1653\gamma^3+333\gamma}{64(\gamma^2-1)^3}\cosh^{-1}\gamma\Bigg]$$

TABLE II. Similar to Table I, but for the component $\mathcal{C}_{\hat{b}}$.

| | |
|---|---|
| $\mathcal{C}_{\hat{b}}^{(0)} = \mathcal{C}_{\hat{b}}^{s_1} = \mathcal{C}_{\hat{b}}^{s_2} = 0$ | |
| $\mathcal{C}_{\hat{b}}^{s_1 s_2}$ | $\frac{(s_1\cdot\hat{b})(s_2\cdot u_1)+(s_1\cdot u_2)(s_2\cdot\hat{b})}{b^2}\Big[-\frac{315\gamma^7-1096\gamma^6-763\gamma^5-15326\gamma^4+69709\gamma^3-120612\gamma^2+103347\gamma-34230}{64(\gamma+1)^3(\gamma^2-1)^{3/2}} + \frac{42\gamma^4+327\gamma^3-273\gamma^2+141\gamma-57}{4(\gamma+1)^2\sqrt{\gamma^2-1}}\log\left(\frac{1+\gamma}{2}\right) - \frac{168\gamma^6+90\gamma^5-324\gamma^4-153\gamma^3+108\gamma^2+27\gamma}{16(\gamma+1)(\gamma^2-1)^2}\cosh^{-1}\gamma\Big]$ |
| $\mathcal{C}_{\hat{b}}^{s_1 s_1}$ | $\frac{(s_1\cdot u_2)(s_1\cdot\hat{b})}{b^2}\Big[-\frac{1575\gamma^8+205\gamma^7-8275\gamma^6+13925\gamma^5-25969\gamma^4+5995\gamma^3-20797\gamma^2+100115\gamma-61494}{640(\gamma+1)^3(\gamma^2-1)^{3/2}} + \frac{147\gamma^4+1044\gamma^3-1014\gamma^2+468\gamma-117}{32(\gamma+1)^2\sqrt{\gamma^2-1}}\log\left(\frac{1+\gamma}{2}\right) - \frac{294\gamma^6+114\gamma^5-603\gamma^4-153\gamma^3+243\gamma^2-27\gamma}{64(\gamma+1)(\gamma^2-1)^2}\cosh^{-1}\gamma\Big]$ $+\frac{C_{E_1}(s_1\cdot u_2)(s_1\cdot\hat{b})}{b^2}\Big[\frac{1575\gamma^8+765\gamma^7+6085\gamma^6+6305\gamma^5+59699\gamma^4-430405\gamma^3+807067\gamma^2-658825\gamma+204374}{640(\gamma+1)^3(\gamma^2-1)^{3/2}} + \frac{147\gamma^4+1044\gamma^3-1014\gamma^2+372\gamma-261}{32(\gamma+1)^2\sqrt{\gamma^2-1}}\log\left(\frac{1+\gamma}{2}\right) - \frac{294\gamma^6+114\gamma^5-603\gamma^4-249\gamma^3+243\gamma^2+117\gamma}{64(\gamma+1)(\gamma^2-1)^2}\cosh^{-1}\gamma\Big]$ |
| $\mathcal{C}_{\hat{b}}^{s_2 s_2}$ | Equal to $-\mathcal{C}_{\hat{b}}^{s_1 s_1}$ after interchanging the body labels $1 \leftrightarrow 2$ |

TABLE III. Similar to Table I, but for the component $\mathcal{C}_{\hat{l}}$.

| | |
|---|---|
| $\mathcal{C}_{\hat{l}}^{(0)}$ | 0 |
| $\mathcal{C}_{\hat{l}}^{s_1}$ | $\frac{(s_1\cdot u_2)}{b}\Big[-\frac{425\gamma^5-1215\gamma^4+2491\gamma^3-3957\gamma^2+2992\gamma-760}{16(\gamma+1)(\gamma^2-1)^2} - \frac{84\gamma^6+459\gamma^5-825\gamma^4-138\gamma^3+666\gamma^2-321\gamma+75}{8(\gamma+1)(\gamma^2-1)^2}\log\left(\frac{1+\gamma}{2}\right) + \frac{168\gamma^7+78\gamma^6-414\gamma^5-171\gamma^4+261\gamma^3+81\gamma^2-27\gamma}{16(\gamma+1)(\gamma^2-1)^{5/2}}\cosh^{-1}\gamma\Big]$ |
| $\mathcal{C}_{\hat{l}}^{s_2}$ | Equal to $\mathcal{C}_{\hat{l}}^{s_1}$ after interchanging the body labels $1 \leftrightarrow 2$ |
| $\mathcal{C}_{\hat{l}}^{s_1 s_2}$ | $\frac{(s_1\cdot\hat{l})(s_2\cdot u_1)+(s_1\cdot u_2)(s_2\cdot\hat{l})}{b^2}\Big[-\frac{315\gamma^6+4714\gamma^5-12807\gamma^4+52652\gamma^3-102963\gamma^2+71562\gamma-16161}{64(\gamma+1)^2(\gamma^2-1)^{3/2}} - \frac{42\gamma^4+327\gamma^3-273\gamma^2+141\gamma-57}{(\gamma+1)^2\sqrt{\gamma^2-1}}\log\left(\frac{1+\gamma}{2}\right) + \frac{168\gamma^6+90\gamma^5-324\gamma^4-153\gamma^3+108\gamma^2+27\gamma}{4(\gamma+1)(\gamma^2-1)^2}\cosh^{-1}\gamma\Big]$ |
| $\mathcal{C}_{\hat{l}}^{s_1 s_1}$ | $\frac{(s_1\cdot u_2)(s_1\cdot\hat{l})}{b^2}\Big[-\frac{1575\gamma^7-4870\gamma^6+19265\gamma^5-36520\gamma^4+222041\gamma^3-461166\gamma^2+316159\gamma-67044}{640(\gamma+1)^2(\gamma^2-1)^{3/2}} - \frac{147\gamma^4+1044\gamma^3-1014\gamma^2+468\gamma-117}{8(\gamma+1)^2\sqrt{\gamma^2-1}}\log\left(\frac{1+\gamma}{2}\right) + \frac{294\gamma^6+114\gamma^5-603\gamma^4-153\gamma^3+243\gamma^2-27\gamma}{16(\gamma+1)(\gamma^2-1)^2}\cosh^{-1}\gamma\Big]$ $+\frac{C_{E_1}(s_1\cdot u_2)(s_1\cdot\hat{l})}{b^2}\Big[\frac{1575\gamma^7-2910\gamma^6-19975\gamma^5+65240\gamma^4-207991\gamma^3+390746\gamma^2-293289\gamma+73324}{640(\gamma+1)^2(\gamma^2-1)^{3/2}} - \frac{147\gamma^4+1044\gamma^3-1014\gamma^2+372\gamma-261}{8(\gamma+1)^2\sqrt{\gamma^2-1}}\log\left(\frac{1+\gamma}{2}\right) + \frac{294\gamma^6+114\gamma^5-603\gamma^4-249\gamma^3+243\gamma^2+117\gamma}{16(\gamma+1)(\gamma^2-1)^2}\cosh^{-1}\gamma\Big]$ |
| $\mathcal{C}_{\hat{l}}^{s_2 s_2}$ | Equal to $\mathcal{C}_{\hat{l}}^{s_1 s_1}$ after interchanging the body labels $1 \leftrightarrow 2$ |

# FEYNMAN RULES

TABLE IV. Momentum-space Feynman rules for the graviton propagator in the de Donder gauge, the worldline vertices corresponding to single- and double-graviton emission from the $A$th body, and the cubic interaction vertex. For the sake of brevity, we write $\mathrm{Sym}[\cdots]$ to denote the action of symmetrizing over all $(\mu_i, \nu_i)$ index pairs; e.g., $\mathrm{Sym}[X^{\mu\nu}] \equiv X^{(\mu\nu)}$ and $\mathrm{Sym}[X^{\mu_1\nu_1\mu_2\nu_2}] \equiv X^{(\mu_1\nu_1)(\mu_2\nu_2)}$. Additionally, we use the shorthands $(U\cdot\mathcal{S}_A\cdot V) \equiv U^\mu \mathcal{S}_{A\,\mu\nu} V^\nu$ and $(U\cdot\mathcal{S}_A\cdot\mathcal{S}_A\cdot V)\equiv U^\mu\mathcal{S}_{A\,\mu\nu}\mathcal{S}_A{}^\nu{}_\rho V^\rho$ to represent the scalar contractions between arbitrary vectors $U$, $V$ and the spin tensor $\mathcal{S}_A$. These rules are valid for generic $d$-dimensional spacetimes.

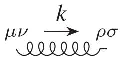


$$\frac{i}{k^2}\left(\eta^{\mu(\rho}\eta^{\sigma)\nu}+\frac{1}{d-2}\eta^{\mu\nu}\eta^{\rho\sigma}\right)$$

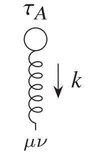


$$\begin{aligned}&-\frac{1}{2}i\kappa\int \mathrm{d}\tau_A\, e^{ik\cdot x_A}\,\mathrm{Sym}\Big[m_A\mathcal{U}_A{}^{\mu}\mathcal{U}_A{}^{\nu}+ik_\rho\mathcal{S}_A{}^{\rho\mu}\mathcal{U}_A{}^{\nu}+\frac{1}{m_A}k_\rho k_\sigma\mathcal{U}_{A\,\alpha}\big(\mathcal{U}_A{}^{\mu}\mathcal{S}_A{}^{\nu\rho}\mathcal{S}_A{}^{\sigma\alpha}+\mathcal{U}_A{}^{\rho}\mathcal{S}_A{}^{\sigma\mu}\mathcal{S}_A{}^{\nu\alpha}\big)\\&+\frac{1}{2m_A}C_{E_A}k_\rho k_\sigma\big(\mathcal{S}_A{}^{\rho\alpha}\mathcal{S}_A{}^{\sigma}{}_{\alpha}\mathcal{U}_A{}^{\mu}\mathcal{U}_A{}^{\nu}+2\mathcal{U}_A{}^{\rho}\mathcal{S}_A{}^{\sigma\alpha}\mathcal{S}_{A\,\alpha}{}^{\mu}\mathcal{U}_A{}^{\nu}+\mathcal{S}_A{}^{\mu}{}_{\alpha}\mathcal{S}_A{}^{\nu\alpha}\mathcal{U}_A{}^{\rho}\mathcal{U}_A{}^{\sigma}\big)\Big]\end{aligned}$$

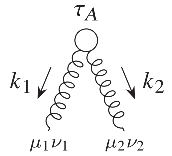


$$\begin{aligned}&\frac{1}{8}i\kappa^2\int\mathrm{d}\tau_A\,e^{i(k_1+k_2)\cdot x_A}\,\mathrm{Sym}\Big[i[(k_1\cdot\mathcal{U}_A)-(k_2\cdot\mathcal{U}_A)]\eta^{\mu_1\mu_2}\mathcal{S}_A{}^{\nu_1\nu_2}-2ik_1{}^{\rho}\eta^{\mu_1\mu_2}\mathcal{S}_A{}^{\nu_2}{}_{\rho}\mathcal{U}_A{}^{\nu_1}-2ik_1{}^{\mu_2}\mathcal{S}_A{}^{\mu_1\nu_2}\mathcal{U}_A{}^{\nu_1}\\
&-2ik_2{}^{\rho}\eta^{\mu_1\mu_2}\mathcal{S}_A{}^{\nu_1}{}_{\rho}\mathcal{U}_A{}^{\nu_2}-2ik_2{}^{\mu_1}\mathcal{S}_A{}^{\mu_2\nu_1}\mathcal{U}_A{}^{\nu_2}+\frac{2}{m_A}\{[(k_1\cdot\mathcal{S}_A\cdot k_2)\mathcal{U}_A{}^{\rho}+k_2{}^{\rho}(k_1\cdot\mathcal{S}_A\cdot\mathcal{U}_A)\\
&+k_2{}^{\rho}(k_2\cdot\mathcal{S}_A\cdot\mathcal{U}_A)]\eta^{\mu_1\mu_2}\mathcal{S}_A{}^{\nu_1}{}_{\rho}\mathcal{U}_A{}^{\nu_2}+[(k_1\cdot\mathcal{S}_A\cdot\mathcal{U}_A)(k_2\cdot\mathcal{U}_A)-(k_1\cdot\mathcal{U}_A)(k_2\cdot\mathcal{S}_A\cdot\mathcal{U}_A)]\eta^{\mu_1\mu_2}\mathcal{S}_A{}^{\nu_1\nu_2}\\
&+[k_1{}^{\rho}(k_1\cdot\mathcal{S}_A\cdot\mathcal{U}_A)+k_1{}^{\rho}(k_2\cdot\mathcal{S}_A\cdot\mathcal{U}_A)-(k_1\cdot\mathcal{S}_A\cdot k_2)\mathcal{U}_A{}^{\rho}]\eta^{\mu_1\mu_2}\mathcal{S}_A{}^{\nu_2}{}_{\rho}\mathcal{U}_A{}^{\nu_1}\\
&+(k_1{}^{\rho}+k_2{}^{\rho})k_1{}^{\mu_2}\mathcal{S}_A{}^{\mu_1}{}_{\rho}\mathcal{S}_A{}^{\nu_2}{}_{\sigma}\mathcal{U}_A{}^{\nu_1}\mathcal{U}_A{}^{\sigma}+[(k_1\cdot\mathcal{S}_A\cdot\mathcal{U}_A)+(k_2\cdot\mathcal{S}_A\cdot\mathcal{U}_A)]k_1{}^{\mu_2}\mathcal{S}_A{}^{\mu_1\nu_2}\mathcal{U}_A{}^{\nu_1}\\
&+(k_1{}^{\rho}+k_2{}^{\rho})k_2{}^{\mu_1}\mathcal{S}_A{}^{\mu_2}{}_{\rho}\mathcal{S}_A{}^{\nu_1}{}_{\sigma}\mathcal{U}_A{}^{\nu_2}\mathcal{U}_A{}^{\sigma}+[(k_1\cdot\mathcal{S}_A\cdot\mathcal{U}_A)+(k_2\cdot\mathcal{S}_A\cdot\mathcal{U}_A)]k_2{}^{\mu_1}\mathcal{S}_A{}^{\mu_2\nu_1}\mathcal{U}_A{}^{\nu_2}\\
&+(k_1{}^{\rho}k_1{}^{\sigma}+k_2{}^{\rho}k_2{}^{\sigma})\mathcal{S}_A{}^{\mu_1}{}_{\rho}\mathcal{S}_A{}^{\mu_2}{}_{\sigma}\mathcal{U}_A{}^{\nu_1}\mathcal{U}_A{}^{\nu_2}+[k_1{}^{\rho}(k_1\cdot\mathcal{U}_A)+(k_1\cdot k_2)\mathcal{U}_A{}^{\rho}]\mathcal{S}_A{}^{\mu_1\mu_2}\mathcal{S}_A{}^{\nu_1}{}_{\rho}\mathcal{U}_A{}^{\nu_2}-[k_1{}^{\rho}(k_1\cdot\mathcal{U}_A)\\
&+k_2{}^{\rho}(k_1\cdot\mathcal{U}_A)+k_2{}^{\rho}(k_2\cdot\mathcal{U}_A)]\eta^{\mu_1\mu_2}\mathcal{S}_A{}^{\nu_1}{}_{\rho}\mathcal{S}_A{}^{\nu_2}{}_{\sigma}\mathcal{U}_A{}^{\sigma}-[k_1{}^{\rho}(k_1\cdot\mathcal{U}_A)+k_1{}^{\rho}(k_2\cdot\mathcal{U}_A)\\
&+k_2{}^{\rho}(k_2\cdot\mathcal{U}_A)]\eta^{\mu_1\mu_2}\mathcal{S}_A{}^{\nu_1}{}_{\sigma}\mathcal{S}_A{}^{\nu_2}{}_{\rho}\mathcal{U}_A{}^{\sigma}-k_1{}^{\rho}k_2{}^{\mu_1}\mathcal{S}_A{}^{\mu_2}{}_{\rho}\mathcal{S}_A{}^{\nu_2}{}_{\sigma}\mathcal{U}_A{}^{\nu_1}\mathcal{U}_A{}^{\sigma}-k_1{}^{\mu_2}k_2{}^{\rho}\mathcal{S}_A{}^{\mu_1}{}_{\rho}\mathcal{S}_A{}^{\nu_1}{}_{\sigma}\mathcal{U}_A{}^{\nu_2}\mathcal{U}_A{}^{\sigma}\\
&-[(k_1\cdot\mathcal{U}_A)+(k_2\cdot\mathcal{U}_A)]k_1{}^{\mu_2}\mathcal{S}_A{}^{\mu_1\nu_2}\mathcal{S}_A{}^{\nu_1}{}_{\rho}\mathcal{U}_A{}^{\rho}-[(k_1\cdot\mathcal{U}_A)+(k_2\cdot\mathcal{U}_A)]k_2{}^{\mu_1}\mathcal{S}_A{}^{\mu_2\nu_1}\mathcal{S}_A{}^{\nu_2}{}_{\rho}\mathcal{U}_A{}^{\rho}\\
&-[(k_1\cdot k_2)\mathcal{U}_A{}^{\rho}+k_2{}^{\rho}(k_2\cdot\mathcal{U}_A)]\mathcal{S}_A{}^{\mu_1\mu_2}\mathcal{S}_A{}^{\nu_2}{}_{\rho}\mathcal{U}_A{}^{\nu_1}\}+\frac{C_{E_A}}{m_A}\{2[k_2{}^{\rho}(k_1\cdot\mathcal{U}_A)-2k_1{}^{\rho}(k_2\cdot\mathcal{U}_A)\\
&-k_2{}^{\rho}(k_2\cdot\mathcal{U}_A)]\eta^{\mu_1\mu_2}\mathcal{S}_A{}^{\nu_1\sigma}\mathcal{S}_{A\,\rho\sigma}\mathcal{U}_A{}^{\nu_2}+2[(k_1\cdot\mathcal{U}_A)^2+(k_1\cdot\mathcal{U}_A)(k_2\cdot\mathcal{U}_A)+(k_2\cdot\mathcal{U}_A)^2]\eta^{\mu_1\mu_2}\mathcal{S}_A{}^{\nu_1\rho}\mathcal{S}_A{}^{\nu_2}{}_{\rho}\\
&+2(k_1{}^{\rho}+k_2{}^{\rho})k_1{}^{\mu_2}\mathcal{S}_A{}^{\nu_2\sigma}\mathcal{S}_{A\,\rho\sigma}\mathcal{U}_A{}^{\mu_1}\mathcal{U}_A{}^{\nu_1}+2(k_2\cdot\mathcal{U}_A)k_1{}^{\mu_2}\mathcal{S}_A{}^{\mu_1\rho}\mathcal{S}_A{}^{\nu_1}{}_{\rho}\mathcal{U}_A{}^{\nu_2}\\
&+2(k_1{}^{\rho}+k_2{}^{\rho})k_2{}^{\mu_1}\mathcal{S}_A{}^{\nu_1\sigma}\mathcal{S}_{A\,\rho\sigma}\mathcal{U}_A{}^{\mu_2}\mathcal{U}_A{}^{\nu_2}+2(k_1\cdot\mathcal{U}_A)k_2{}^{\mu_1}\mathcal{S}_A{}^{\mu_2\rho}\mathcal{S}_A{}^{\nu_2}{}_{\rho}\mathcal{U}_A{}^{\nu_1}+2(k_1\cdot k_2)\mathcal{S}_A{}^{\mu_1\rho}\mathcal{S}_A{}^{\mu_2}{}_{\rho}\mathcal{U}_A{}^{\nu_1}\mathcal{U}_A{}^{\nu_2}\\
&-2[2k_2{}^{\rho}(k_1\cdot\mathcal{U}_A)+k_1{}^{\rho}(k_1\cdot\mathcal{U}_A)-k_1{}^{\rho}(k_2\cdot\mathcal{U}_A)]\eta^{\mu_1\mu_2}\mathcal{S}_A{}^{\nu_2\sigma}\mathcal{S}_{A\,\rho\sigma}\mathcal{U}_A{}^{\nu_1}-2(k_1\cdot\mathcal{S}_A\cdot\mathcal{S}_A\cdot k_2)\eta^{\mu_1\mu_2}\mathcal{U}_A{}^{\nu_1}\mathcal{U}_A{}^{\nu_2}\\
&-2k_1{}^{\rho}k_2{}^{\mu_1}\mathcal{S}_A{}^{\mu_2\sigma}\mathcal{S}_{A\,\rho\sigma}\mathcal{U}_A{}^{\nu_1}\mathcal{U}_A{}^{\nu_2}-2k_1{}^{\mu_2}k_2{}^{\rho}\mathcal{S}_A{}^{\mu_1\sigma}\mathcal{S}_{A\,\rho\sigma}\mathcal{U}_A{}^{\nu_1}\mathcal{U}_A{}^{\nu_2}\\
&-2[(k_1\cdot\mathcal{U}_A)+(k_2\cdot\mathcal{U}_A)]k_1{}^{\mu_2}\mathcal{S}_A{}^{\mu_1\rho}\mathcal{S}_A{}^{\nu_2}{}_{\rho}\mathcal{U}_A{}^{\nu_1}-2[(k_1\cdot\mathcal{U}_A)+(k_2\cdot\mathcal{U}_A)]k_2{}^{\mu_1}\mathcal{S}_A{}^{\mu_2\rho}\mathcal{S}_A{}^{\nu_1}{}_{\rho}\mathcal{U}_A{}^{\nu_2}\\
&-(k_1\cdot k_2)\mathcal{S}_A{}^{\mu_1\rho}\mathcal{S}_A{}^{\nu_1}{}_{\rho}\mathcal{U}_A{}^{\mu_2}\mathcal{U}_A{}^{\nu_2}-(k_1\cdot k_2)\mathcal{S}_A{}^{\mu_2\rho}\mathcal{S}_A{}^{\nu_2}{}_{\rho}\mathcal{U}_A{}^{\mu_1}\mathcal{U}_A{}^{\nu_1}\}\Big]\end{aligned}$$

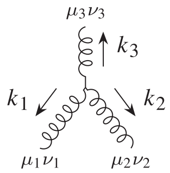


$$\begin{aligned}&\tfrac{1}{8}i\kappa\,\mathrm{Sym}\,\big[10k_1^2\eta^{\mu_1\mu_2}\eta^{\mu_3\nu_3}\eta^{\nu_1\nu_2}+16(k_1\cdot k_2)\eta^{\mu_1\mu_2}\eta^{\mu_3\nu_3}\eta^{\nu_1\nu_2}+2(k_1\cdot k_3)\eta^{\mu_1\mu_2}\eta^{\mu_3\nu_3}\eta^{\nu_1\nu_2}+10k_2^2\eta^{\mu_1\mu_2}\eta^{\mu_3\nu_3}\eta^{\nu_1\nu_2}\\
&+2(k_2\cdot k_3)\eta^{\mu_1\mu_2}\eta^{\mu_3\nu_3}\eta^{\nu_1\nu_2}+10k_1^2\eta^{\mu_1\mu_3}\eta^{\mu_2\nu_2}\eta^{\nu_1\nu_3}+2(k_1\cdot k_2)\eta^{\mu_1\mu_3}\eta^{\mu_2\nu_2}\eta^{\nu_1\nu_3}+16(k_1\cdot k_3)\eta^{\mu_1\mu_3}\eta^{\mu_2\nu_2}\eta^{\nu_1\nu_3}\\
&+2(k_2\cdot k_3)\eta^{\mu_1\mu_3}\eta^{\mu_2\nu_2}\eta^{\nu_1\nu_3}+10k_3^2\eta^{\mu_1\mu_3}\eta^{\mu_2\nu_2}\eta^{\nu_1\nu_3}+2(k_1\cdot k_2)\eta^{\mu_1\nu_1}\eta^{\mu_2\mu_3}\eta^{\nu_2\nu_3}+2(k_1\cdot k_3)\eta^{\mu_1\nu_1}\eta^{\mu_2\mu_3}\eta^{\nu_2\nu_3}\\
&+10k_2^2\eta^{\mu_1\nu_1}\eta^{\mu_2\mu_3}\eta^{\nu_2\nu_3}+16(k_2\cdot k_3)\eta^{\mu_1\nu_1}\eta^{\mu_2\mu_3}\eta^{\nu_2\nu_3}+10k_3^2\eta^{\mu_1\nu_1}\eta^{\mu_2\mu_3}\eta^{\nu_2\nu_3}+9k_1{}^{\mu_1}k_1{}^{\mu_2}\eta^{\mu_3\nu_1}\eta^{\nu_2\nu_3}\\
&+15k_1{}^{\mu_1}k_1{}^{\mu_2}\eta^{\mu_3\nu_2}\eta^{\nu_1\nu_3}+12k_1{}^{\mu_1}k_1{}^{\mu_3}\eta^{\mu_2\nu_1}\eta^{\nu_2\nu_3}+12k_1{}^{\mu_1}k_1{}^{\mu_3}\eta^{\mu_2\nu_3}\eta^{\nu_1\nu_2}+16k_1{}^{\mu_1}k_1{}^{\nu_1}\eta^{\mu_2\nu_2}\eta^{\mu_3\nu_3}\\
&+20k_1{}^{\mu_1}k_2{}^{\mu_2}\eta^{\mu_3\nu_1}\eta^{\nu_2\nu_3}+12k_1{}^{\mu_1}k_2{}^{\mu_2}\eta^{\mu_3\nu_2}\eta^{\nu_1\nu_3}+12k_1{}^{\mu_1}k_2{}^{\mu_3}\eta^{\mu_2\nu_1}\eta^{\nu_2\nu_3}+4k_1{}^{\mu_1}k_2{}^{\mu_3}\eta^{\mu_2\nu_3}\eta^{\nu_1\nu_2}\\
&+12k_1{}^{\mu_1}k_2{}^{\nu_1}\eta^{\mu_2\nu_2}\eta^{\mu_3\nu_3}+10k_1{}^{\mu_1}k_3{}^{\mu_2}\eta^{\mu_3\nu_1}\eta^{\nu_2\nu_3}+6k_1{}^{\mu_1}k_3{}^{\mu_2}\eta^{\mu_3\nu_2}\eta^{\nu_1\nu_3}+24k_1{}^{\mu_1}k_3{}^{\mu_3}\eta^{\mu_2\nu_1}\eta^{\nu_2\nu_3}\\
&+8k_1{}^{\mu_1}k_3{}^{\mu_3}\eta^{\mu_2\nu_3}\eta^{\nu_1\nu_2}+12k_1{}^{\mu_1}k_3{}^{\nu_1}\eta^{\mu_2\nu_2}\eta^{\mu_3\nu_3}+4k_1{}^{\mu_2}k_1{}^{\nu_2}\eta^{\mu_1\mu_3}\eta^{\nu_1\nu_3}+4k_1{}^{\mu_2}k_2{}^{\mu_3}\eta^{\mu_1\nu_1}\eta^{\nu_2\nu_3}\\
&+12k_1{}^{\mu_2}k_2{}^{\nu_2}\eta^{\mu_1\nu_1}\eta^{\mu_3\nu_3}+4k_1{}^{\mu_2}k_3{}^{\mu_1}\eta^{\mu_3\nu_3}\eta^{\nu_1\nu_2}+8k_1{}^{\mu_2}k_3{}^{\mu_3}\eta^{\mu_1\nu_2}\eta^{\nu_1\nu_3}+8k_1{}^{\mu_2}k_3{}^{\mu_3}\eta^{\mu_1\nu_3}\eta^{\nu_1\nu_2}\end{aligned}$$

$$
\begin{aligned}
&+16{k_1}^{\mu_2}{k_3}^{\nu_2}\eta^{\mu_1\mu_3}\eta^{\nu_1\nu_3}+4{k_1}^{\mu_3}{k_1}^{\nu_3}\eta^{\mu_1\mu_2}\eta^{\nu_1\nu_2}+4{k_1}^{\mu_3}{k_2}^{\mu_1}\eta^{\mu_2\nu_2}\eta^{\nu_1\nu_3}+8{k_1}^{\mu_3}{k_2}^{\mu_2}\eta^{\mu_1\nu_2}\eta^{\nu_1\nu_3}\\
&+8{k_1}^{\mu_3}{k_2}^{\mu_2}\eta^{\mu_1\nu_3}\eta^{\nu_1\nu_2}+16{k_1}^{\mu_3}{k_2}^{\nu_3}\eta^{\mu_1\mu_2}\eta^{\nu_1\nu_2}+4{k_1}^{\mu_3}{k_3}^{\mu_2}\eta^{\mu_1\nu_1}\eta^{\nu_2\nu_3}+12{k_1}^{\mu_3}{k_3}^{\nu_3}\eta^{\mu_1\nu_1}\eta^{\mu_2\nu_2}\\
&+9{k_2}^{\mu_1}{k_2}^{\mu_2}\eta^{\mu_3\nu_1}\eta^{\nu_2\nu_3}+15{k_2}^{\mu_1}{k_2}^{\mu_2}\eta^{\mu_3\nu_2}\eta^{\nu_1\nu_3}+4{k_2}^{\mu_1}{k_2}^{\nu_1}\eta^{\mu_2\mu_3}\eta^{\nu_2\nu_3}+4{k_2}^{\mu_1}{k_3}^{\mu_2}\eta^{\mu_3\nu_3}\eta^{\nu_1\nu_2}\\
&+12{k_2}^{\mu_1}{k_3}^{\mu_3}\eta^{\mu_2\nu_1}\eta^{\nu_2\nu_3}+4{k_2}^{\mu_1}{k_3}^{\mu_3}\eta^{\mu_2\nu_3}\eta^{\nu_1\nu_2}+16{k_2}^{\mu_1}{k_3}^{\nu_1}\eta^{\mu_2\mu_3}\eta^{\nu_2\nu_3}+12{k_2}^{\mu_2}{k_2}^{\mu_3}\eta^{\mu_1\nu_2}\eta^{\nu_1\nu_3}\\
&+12{k_2}^{\mu_2}{k_2}^{\mu_3}\eta^{\mu_1\nu_3}\eta^{\nu_1\nu_2}+16{k_2}^{\mu_2}{k_2}^{\nu_2}\eta^{\mu_1\nu_1}\eta^{\mu_3\nu_3}+10{k_2}^{\mu_2}{k_3}^{\mu_1}\eta^{\mu_3\nu_1}\eta^{\nu_2\nu_3}+6{k_2}^{\mu_2}{k_3}^{\mu_1}\eta^{\mu_3\nu_2}\eta^{\nu_1\nu_3}\\
&+16{k_2}^{\mu_2}{k_3}^{\mu_3}\eta^{\mu_1\nu_2}\eta^{\nu_1\nu_3}+16{k_2}^{\mu_2}{k_3}^{\mu_3}\eta^{\mu_1\nu_3}\eta^{\nu_1\nu_2}+12{k_2}^{\mu_2}{k_3}^{\nu_2}\eta^{\mu_1\nu_1}\eta^{\mu_3\nu_3}+4{k_2}^{\mu_3}{k_2}^{\nu_3}\eta^{\mu_1\mu_2}\eta^{\nu_1\nu_2}\\
&+4{k_2}^{\mu_3}{k_3}^{\mu_1}\eta^{\mu_2\nu_2}\eta^{\nu_1\nu_3}+12{k_2}^{\mu_3}{k_3}^{\nu_3}\eta^{\mu_1\nu_1}\eta^{\mu_2\nu_2}+12{k_3}^{\mu_1}{k_3}^{\mu_3}\eta^{\mu_2\nu_1}\eta^{\nu_2\nu_3}+12{k_3}^{\mu_1}{k_3}^{\mu_3}\eta^{\mu_2\nu_3}\eta^{\nu_1\nu_2}\\
&+4{k_3}^{\mu_1}{k_3}^{\nu_1}\eta^{\mu_2\mu_3}\eta^{\nu_2\nu_3}+12{k_3}^{\mu_2}{k_3}^{\mu_3}\eta^{\mu_1\nu_2}\eta^{\nu_1\nu_3}+12{k_3}^{\mu_2}{k_3}^{\mu_3}\eta^{\mu_1\nu_3}\eta^{\nu_1\nu_2}+4{k_3}^{\mu_2}{k_3}^{\nu_2}\eta^{\mu_1\mu_3}\eta^{\nu_1\nu_3}\\
&+16{k_3}^{\mu_3}{k_3}^{\nu_3}\eta^{\mu_1\nu_1}\eta^{\mu_2\nu_2}-6k_1^2\eta^{\mu_1\mu_2}\eta^{\mu_3\nu_1}\eta^{\nu_2\nu_3}-6(k_1\cdot k_2)\eta^{\mu_1\mu_2}\eta^{\mu_3\nu_1}\eta^{\nu_2\nu_3}-6(k_1\cdot k_3)\eta^{\mu_1\mu_2}\eta^{\mu_3\nu_1}\eta^{\nu_2\nu_3}\\
&-6k_2^2\eta^{\mu_1\mu_2}\eta^{\mu_3\nu_1}\eta^{\nu_2\nu_3}-6(k_2\cdot k_3)\eta^{\mu_1\mu_2}\eta^{\mu_3\nu_1}\eta^{\nu_2\nu_3}-6k_3^2\eta^{\mu_1\mu_2}\eta^{\mu_3\nu_1}\eta^{\nu_2\nu_3}-10k_1^2\eta^{\mu_1\mu_2}\eta^{\mu_3\nu_2}\eta^{\nu_1\nu_3}\\
&-10(k_1\cdot k_2)\eta^{\mu_1\mu_2}\eta^{\mu_3\nu_2}\eta^{\nu_1\nu_3}-10(k_1\cdot k_3)\eta^{\mu_1\mu_2}\eta^{\mu_3\nu_2}\eta^{\nu_1\nu_3}-10k_2^2\eta^{\mu_1\mu_2}\eta^{\mu_3\nu_2}\eta^{\nu_1\nu_3}-10(k_2\cdot k_3)\eta^{\mu_1\mu_2}\eta^{\mu_3\nu_2}\eta^{\nu_1\nu_3}\\
&-10k_3^2\eta^{\mu_1\mu_2}\eta^{\mu_3\nu_2}\eta^{\nu_1\nu_3}-4k_1^2\eta^{\mu_1\nu_1}\eta^{\mu_2\nu_2}\eta^{\mu_3\nu_3}-4(k_1\cdot k_2)\eta^{\mu_1\nu_1}\eta^{\mu_2\nu_2}\eta^{\mu_3\nu_3}-4(k_1\cdot k_3)\eta^{\mu_1\nu_1}\eta^{\mu_2\nu_2}\eta^{\mu_3\nu_3}\\
&-4k_2^2\eta^{\mu_1\nu_1}\eta^{\mu_2\nu_2}\eta^{\mu_3\nu_3}-4(k_2\cdot k_3)\eta^{\mu_1\nu_1}\eta^{\mu_2\nu_2}\eta^{\mu_3\nu_3}-4k_3^2\eta^{\mu_1\nu_1}\eta^{\mu_2\nu_2}\eta^{\mu_3\nu_3}-20{k_1}^{\mu_1}{k_1}^{\mu_2}\eta^{\mu_3\nu_3}\eta^{\nu_1\nu_2}\\
&-20{k_1}^{\mu_1}{k_1}^{\mu_3}\eta^{\mu_2\nu_2}\eta^{\nu_1\nu_3}-32{k_1}^{\mu_1}{k_1}^{\nu_1}\eta^{\mu_2\mu_3}\eta^{\nu_2\nu_3}-32{k_1}^{\mu_1}{k_2}^{\mu_2}\eta^{\mu_3\nu_3}\eta^{\nu_1\nu_2}-8{k_1}^{\mu_1}{k_2}^{\mu_3}\eta^{\mu_2\nu_2}\eta^{\nu_1\nu_3}\\
&-20{k_1}^{\mu_1}{k_2}^{\nu_1}\eta^{\mu_2\mu_3}\eta^{\nu_2\nu_3}-8{k_1}^{\mu_1}{k_3}^{\mu_2}\eta^{\mu_3\nu_3}\eta^{\nu_1\nu_2}-32{k_1}^{\mu_1}{k_3}^{\mu_3}\eta^{\mu_2\nu_2}\eta^{\nu_1\nu_3}-20{k_1}^{\mu_1}{k_3}^{\nu_1}\eta^{\mu_2\mu_3}\eta^{\nu_2\nu_3}\\
&-4{k_1}^{\mu_2}{k_2}^{\mu_3}\eta^{\mu_1\nu_2}\eta^{\nu_1\nu_3}-4{k_1}^{\mu_2}{k_2}^{\mu_3}\eta^{\mu_1\nu_3}\eta^{\nu_1\nu_2}-20{k_1}^{\mu_2}{k_2}^{\nu_2}\eta^{\mu_1\mu_3}\eta^{\nu_1\nu_3}-5{k_1}^{\mu_2}{k_3}^{\mu_1}\eta^{\mu_3\nu_1}\eta^{\nu_2\nu_3}\\
&-3{k_1}^{\mu_2}{k_3}^{\mu_1}\eta^{\mu_3\nu_2}\eta^{\nu_1\nu_3}-8{k_1}^{\mu_2}{k_3}^{\mu_3}\eta^{\mu_1\nu_1}\eta^{\nu_2\nu_3}-8{k_1}^{\mu_2}{k_3}^{\nu_2}\eta^{\mu_1\nu_1}\eta^{\mu_3\nu_3}-6{k_1}^{\mu_3}{k_2}^{\mu_1}\eta^{\mu_2\nu_1}\eta^{\nu_2\nu_3}\\
&-2{k_1}^{\mu_3}{k_2}^{\mu_1}\eta^{\mu_2\nu_3}\eta^{\nu_1\nu_2}-8{k_1}^{\mu_3}{k_2}^{\mu_2}\eta^{\mu_1\nu_1}\eta^{\nu_2\nu_3}-8{k_1}^{\mu_3}{k_2}^{\nu_3}\eta^{\mu_1\nu_1}\eta^{\mu_2\nu_2}-4{k_1}^{\mu_3}{k_3}^{\mu_2}\eta^{\mu_1\nu_2}\eta^{\nu_1\nu_3}\\
&-4{k_1}^{\mu_3}{k_3}^{\mu_2}\eta^{\mu_1\nu_3}\eta^{\nu_1\nu_2}-20{k_1}^{\mu_3}{k_3}^{\nu_3}\eta^{\mu_1\mu_2}\eta^{\nu_1\nu_2}-20{k_2}^{\mu_1}{k_2}^{\mu_2}\eta^{\mu_3\nu_3}\eta^{\nu_1\nu_2}-5{k_2}^{\mu_1}{k_3}^{\mu_2}\eta^{\mu_3\nu_1}\eta^{\nu_2\nu_3}\\
&-3{k_2}^{\mu_1}{k_3}^{\mu_2}\eta^{\mu_3\nu_2}\eta^{\nu_1\nu_3}-8{k_2}^{\mu_1}{k_3}^{\mu_3}\eta^{\mu_2\nu_2}\eta^{\nu_1\nu_3}-8{k_2}^{\mu_1}{k_3}^{\nu_1}\eta^{\mu_2\nu_2}\eta^{\mu_3\nu_3}-20{k_2}^{\mu_2}{k_2}^{\mu_3}\eta^{\mu_1\nu_1}\eta^{\nu_2\nu_3}\\
&-32{k_2}^{\mu_2}{k_2}^{\nu_2}\eta^{\mu_1\mu_3}\eta^{\nu_1\nu_3}-8{k_2}^{\mu_2}{k_3}^{\mu_1}\eta^{\mu_3\nu_3}\eta^{\nu_1\nu_2}-32{k_2}^{\mu_2}{k_3}^{\mu_3}\eta^{\mu_1\nu_1}\eta^{\nu_2\nu_3}-20{k_2}^{\mu_2}{k_3}^{\nu_2}\eta^{\mu_1\mu_3}\eta^{\nu_1\nu_3}\\
&-6{k_2}^{\mu_3}{k_3}^{\mu_1}\eta^{\mu_2\nu_1}\eta^{\nu_2\nu_3}-2{k_2}^{\mu_3}{k_3}^{\mu_1}\eta^{\mu_2\nu_3}\eta^{\nu_1\nu_2}-20{k_2}^{\mu_3}{k_3}^{\nu_3}\eta^{\mu_1\mu_2}\eta^{\nu_1\nu_2}-20{k_3}^{\mu_1}{k_3}^{\mu_3}\eta^{\mu_2\nu_2}\eta^{\nu_1\nu_3}\\
&-20{k_3}^{\mu_2}{k_3}^{\mu_3}\eta^{\mu_1\nu_1}\eta^{\nu_2\nu_3}-32{k_3}^{\mu_3}{k_3}^{\nu_3}\eta^{\mu_1\mu_2}\eta^{\nu_1\nu_2}\Big]
\end{aligned}
$$

## DEFLECTIONS IN THE TRAJECTORIES

TABLE V. Deflections $\delta^{(1)}X_1(\tau_1)$ for the body variables $X_1 \equiv (x_1^\mu, \mathcal{U}_1^\mu, \mathcal{S}_1^{\mu\nu})$ at first order in $G$ and up to quadratic order in the spins. The corresponding deflections for the second body can be obtained by interchanging the body labels $1 \leftrightarrow 2$. For the sake of brevity, the operator Asym$[\cdots]$ denotes the action of antisymmetrizing over the indices $(\mu, \nu)$; we use the shorthands $(U \cdot s_A \cdot V) \equiv U^\mu s_{A\,\mu\nu} V^\nu$ and $(U \cdot s_A \cdot s_B \cdot V) \equiv U^\mu s_{A\,\mu\nu} {s_B}^\nu{}_\rho V^\rho$ to represent the scalar contractions between arbitrary vectors $U$, $V$ and the reduced spin tensors $s_A$; and we write $\beta_\gamma \equiv \gamma^2 - 1/(d-2)$. These results are valid in generic $d$-dimensional spacetimes. When used to compute the stress-energy tensor at next-to-leading order in $G$, one should rename the momentum variable $\ell$ that is being integrated over to $k - q$ in the case of body 1, and to $q$ in the case of body 2, so as to be consistent with the definition of $q$ in Table VI and in the main text. Strictly, one should also shift the inner product $(\ell \cdot u_1) \to (\ell \cdot u_1) + i0^+$ in order to satisfy the initial condition $\delta^{(1)}X_1(-\infty) = 0$, but this $i0^+$ part does not otherwise affect our final result for the stress-energy tensor, and so has not been written out explicitly.

$\delta^{(1)}x_1^\mu(\tau_1)$

$$
\begin{aligned}
&\frac{i\kappa^2 m_2}{4}\int_\ell \frac{e^{-i\ell\cdot(b+u_1\tau_1)}}{\ell^2(\ell\cdot u_1)}\,\delta(\ell\cdot u_2)\Bigg[\frac{\beta_\gamma}{(\ell\cdot u_1)}\ell^\mu-\frac{2}{d-2}{u_1}^\mu-2\gamma {u_2}^\mu+i\bigg(\gamma\ell^\nu {s_2}^\mu{}_\nu+\frac{\gamma}{(\ell\cdot u_1)}[(\ell\cdot s_2\cdot u_1)-(\ell\cdot s_1\cdot u_2)]\ell^\mu\\
&+[(\ell\cdot s_1\cdot u_2)-(\ell\cdot s_2\cdot u_1)]{u_2}^\mu-\frac{1}{d-2}\ell^\nu {s_1}^\mu{}_\nu\bigg)+\frac{2(\ell\cdot u_1)}{d-2}(1+C_{E_1})\ell^\nu {s_1}^{\mu\rho}s_{1\,\nu\rho}+(\ell\cdot s_1\cdot u_2)\ell^\nu {s_2}^\mu{}_\nu\\
&+\frac{1}{(d-2)(\ell\cdot u_1)}[2(\ell\cdot s_1\cdot u_2)(\ell\cdot s_2\cdot u_1)+\beta_\gamma C_{E_2}d(\ell\cdot s_2\cdot s_2\cdot\ell)+C_{E_1}(d-2)(\ell\cdot u_1)^2(u_2\cdot s_1\cdot s_1\cdot u_2)\\
&-2\beta_\gamma C_{E_2}(\ell\cdot s_2\cdot s_2\cdot\ell)-\beta_\gamma C_{E_1}(d-2)(\ell\cdot s_1\cdot s_1\cdot\ell)-C_{E_1}(\ell\cdot u_1)^2(s_{1\,\nu\rho}{s_1}^{\nu\rho})-d(\ell\cdot s_1\cdot u_2)(\ell\cdot s_2\cdot u_1)\\
&-\gamma(d-2)(\ell\cdot s_1\cdot s_2\cdot\ell)]\ell^\mu+2(\ell\cdot s_1\cdot u_2)[(\ell\cdot u_1){u_2}^\nu-\gamma\ell^\nu]{s_1}^\mu{}_\nu+\frac{2}{d-2}[C_{E_1}(\ell\cdot s_1\cdot s_1\cdot\ell)+C_{E_2}(\ell\cdot s_2\cdot s_2\cdot\ell)]{u_1}^\mu
\end{aligned}
$$

$$+ [2\gamma C_{E_1}(\ell\cdot s_1\cdot s_1\cdot\ell) + 2\gamma C_{E_2}(\ell\cdot s_2\cdot s_2\cdot\ell) + (\ell\cdot s_1\cdot s_2\cdot\ell) - 2C_{E_1}(\ell\cdot u_1)(\ell\cdot s_1\cdot s_1\cdot u_2)]{u_2}^\mu\Big]$$

$\delta^{(1)}\mathcal{U}_1^\mu(\tau_1)$ Can be obtained by differentiating $\delta^{(1)}x_1^\mu$ with respect to $\tau_1$, which simply adds a factor of $-i(\ell\cdot u_1)$ to the integrand

$\delta^{(1)}\mathcal{S}_1^{\mu\nu}(\tau_1)$

$$-\frac{\kappa^2 m_1 m_2}{4}\int_\ell \frac{e^{-i\ell\cdot(b+u_1\tau_1)}}{\ell^2(\ell\cdot u_1)}\delta(\ell\cdot u_2)\,\mathrm{Asym}\Bigg[\frac{2}{d-2}\ell^\rho {s_1}^\mu{}_\rho {u_1}^\nu + 2\gamma\ell^\rho {s_1}^\mu{}_\rho {u_2}^\nu + 2\gamma\ell^\mu {s_1}^\nu{}_\rho {u_2}^\rho$$
$$+ i\bigg(\frac{4(\ell\cdot u_1)}{d-2}(1+C_{E_1})\ell^\rho {s_1}^{\mu\sigma} s_{1\,\rho\sigma}{u_1}^\nu + 2(\ell\cdot s_2\cdot u_1)\ell^\rho {s_1}^\mu{}_\rho {u_2}^\nu + 2(\ell\cdot s_2\cdot u_1)\ell^\mu {s_1}^\nu{}_\rho {u_2}^\rho + [2\gamma\ell^\rho s_{2\,\rho\sigma}$$
$$+ 4\beta_\gamma C_{E_1}\ell^\rho s_{1\,\rho\sigma} - 4\gamma C_{E_1} s_{1\,\rho\sigma}(\ell\cdot u_1){u_2}^\rho]\ell^\mu {s_1}^{\nu\sigma} + 4C_{E_1}(\ell\cdot u_1)[\gamma\ell^\rho - (\ell\cdot u_1){u_2}^\rho]{s_1}^{\mu\sigma}s_{1\,\rho\sigma}{u_2}^\nu$$
$$+ 4(\ell\cdot s_1\cdot u_2)[(\ell\cdot u_1){u_2}^\rho - \gamma\ell^\rho]{s_1}^\mu{}_\rho {u_1}^\nu - 2\gamma\ell^\rho\ell^\sigma {s_1}^\mu{}_\rho {s_2}^\nu{}_\sigma\bigg)\Bigg]$$

## STRESS-ENERGY TENSOR

TABLE VI. The integrand $t^{\mu\nu}$ in the stress-energy tensor at next-to-leading order in $G$. We organize this result in powers of the spins by writing $t = t_{(0)} + \Sigma_{A=1}^2 t_{s_A} + \Sigma_{A=1}^2\Sigma_{B=A}^2 t_{s_A s_B} + O(s^3)$, where the subscript (0) denotes the part that is independent of the spins, the subscript $s_1$ denotes the part that is proportional to $s_1$, and so on. As in previous tables, Sym$[\cdots]$ denotes a symmetrization over the free indices $(\mu,\nu)$; we use the shorthands $(U\cdot s_A\cdot V)\equiv U^\mu s_{A\,\mu\nu}V^\nu$ and $(U\cdot s_A\cdot s_B\cdot V)\equiv U^\mu s_{A\,\mu\nu}{s_B}^\nu{}_\rho V^\rho$ to represent the scalar contractions between arbitrary vectors $U, V$ and the reduced spin tensors $s_A$; and we write $\beta_\gamma\equiv\gamma^2 - 1/(d-2)$ for the sake of brevity. As $k^2=0$ on shell, terms proportional to $k^2$ do not contribute to the radiated momentum and so have not been included. This result is valid for generic $d$-dimensional spacetimes.

$t^{\mu\nu}_{(0)}$

$$\mathrm{Sym}\Bigg[\frac{1}{d-2}[2\gamma(d-2)(k\cdot u_1)(k\cdot u_2) + 2(k\cdot u_1)^2 + 2(k\cdot u_2)^2 + \beta_\gamma(d-2)(k\cdot q) - \beta_\gamma(d-2)q^2]\eta^{\mu\nu} + 2\beta_\gamma k^\mu k^\nu$$
$$+ \frac{1}{(d-2)(k\cdot u_1)}[2\beta_\gamma(d-2)q^2 - 4(k\cdot u_1)^2]k^\mu {u_1}^\nu + 2\beta_\gamma q^\mu q^\nu + \frac{1}{(k\cdot u_2)}[2\beta_\gamma q^2 + 4\gamma(k\cdot u_1)(k\cdot u_2) - 4\beta_\gamma(k\cdot q)]q^\mu {u_2}^\nu$$
$$+ \frac{1}{(k\cdot u_1)^2}[2\gamma(k\cdot u_1)(k\cdot u_2)q^2 + 2(k\cdot u_1)^2(k\cdot u_2)^2 + \beta_\gamma(k\cdot q)q^2]{u_1}^\mu {u_1}^\nu + [4\gamma(k\cdot q) - 4\gamma q^2 - 4(k\cdot u_1)(k\cdot u_2)]{u_1}^\mu {u_2}^\nu$$
$$+ \frac{1}{(k\cdot u_2)^2}[2\beta_\gamma(k\cdot q)^2 + 2\gamma(k\cdot u_1)(k\cdot u_2)q^2 + 2(k\cdot u_1)^2(k\cdot u_2)^2 - 4\gamma(k\cdot q)(k\cdot u_1)(k\cdot u_2) - \beta_\gamma(k\cdot q)q^2]{u_2}^\mu {u_2}^\nu - 2\beta_\gamma k^\mu q^\nu$$
$$- \frac{4}{d-2}[\gamma(d-2)(k\cdot u_1) + (k\cdot u_2)]k^\mu {u_2}^\nu - \frac{2}{(k\cdot u_1)}[2\gamma(k\cdot u_1)(k\cdot u_2) + \beta_\gamma q^2]q^\mu {u_1}^\nu\Bigg]$$

$t^{\mu\nu}_{s_1}$

$$i\,\mathrm{Sym}\Bigg[\frac{1}{d-2}[(d-2)(k\cdot u_1)(k\cdot u_2)(q\cdot s_1\cdot u_2) + \gamma(d-2)(k\cdot q)(q\cdot s_1\cdot u_2) - 2(k\cdot u_1)(k\cdot s_1\cdot q) - \gamma(d-2)(k\cdot u_2)(k\cdot s_1\cdot q)$$
$$- \gamma(d-2)(q\cdot s_1\cdot u_2)q^2]\eta^{\mu\nu} + 2\gamma(q\cdot s_1\cdot u_2)k^\mu k^\nu + \frac{1}{(d-2)(k\cdot u_1)}[2q^\rho(k\cdot u_1)^2 + \gamma(d-2)(k\cdot u_1)q^2{u_2}^\rho$$
$$- \beta_\gamma(d-2)k^\rho q^2]k^\mu {s_1}^\nu{}_\rho + \frac{1}{(d-2)(k\cdot u_1)}[2\gamma(d-2)(q\cdot s_1\cdot u_2)q^2 + 2(k\cdot u_1)(k\cdot s_1\cdot q) - \gamma(d-2)(k\cdot s_1\cdot u_2)q^2]k^\mu {u_1}^\nu$$
$$+ [2\gamma(k\cdot s_1\cdot q) - 2(k\cdot u_1)(q\cdot s_1\cdot u_2)]k^\mu {u_2}^\nu + 2\gamma(q\cdot s_1\cdot u_2)q^\mu q^\nu + \frac{1}{(k\cdot u_1)}[2\gamma q^\rho(k\cdot u_1)(k\cdot u_2) + \beta_\gamma k^\rho q^2$$
$$- \gamma(k\cdot u_1)q^2{u_2}^\rho]q^\mu {s_1}^\nu{}_\rho + \frac{1}{(k\cdot u_1)}[\gamma(k\cdot s_1\cdot u_2)q^2 - 2\gamma(q\cdot s_1\cdot u_2)q^2 - 2(k\cdot u_1)(k\cdot u_2)(q\cdot s_1\cdot u_2)]q^\mu {u_1}^\nu$$
$$+ \frac{1}{(k\cdot u_2)}[2\gamma(q\cdot s_1\cdot u_2)q^2 + 2(k\cdot u_1)(k\cdot u_2)(q\cdot s_1\cdot u_2) - 2\gamma(k\cdot u_2)(k\cdot s_1\cdot q) - 4\gamma(k\cdot q)(q\cdot s_1\cdot u_2)]q^\mu {u_2}^\nu$$
$$+ \frac{1}{(k\cdot u_1)^2}[\gamma(k\cdot q)(k\cdot u_1)q^2{u_2}^\rho + (k\cdot u_1)^2(k\cdot u_2)q^2{u_2}^\rho - 2q^\rho(k\cdot u_1)^2(k\cdot u_2)^2 - \beta_\gamma k^\rho(k\cdot q)q^2 - \gamma k^\rho(k\cdot u_1)(k\cdot u_2)q^2$$
$$- \gamma q^\rho(k\cdot u_1)(k\cdot u_2)q^2]{s_1}^\mu{}_\rho {u_1}^\nu + [2q^\rho(k\cdot u_1)(k\cdot u_2) + \gamma k^\rho q^2 + \gamma q^\rho q^2 - 2\gamma q^\rho(k\cdot q) - (k\cdot u_1)q^2{u_2}^\rho]{s_1}^\mu{}_\rho {u_2}^\nu$$

$$
\begin{aligned}
&+\frac{1}{(k\cdot u_1)}[2(k\cdot q)(k\cdot u_1)(q\cdot s_1\cdot u_2)+2(k\cdot u_1)(k\cdot u_2)(k\cdot s_1\cdot q)+\gamma(k\cdot s_1\cdot q)q^2+(k\cdot u_1)(k\cdot s_1\cdot u_2)q^2\\
&-2(k\cdot u_1)(q\cdot s_1\cdot u_2)q^2]{u_1}^{\mu}{u_2}^{\nu}+\frac{1}{(k\cdot u_2)^2}[2\gamma(k\cdot q)^2(q\cdot s_1\cdot u_2)+2\gamma(k\cdot q)(k\cdot u_2)(k\cdot s_1\cdot q)+(k\cdot u_1)(k\cdot u_2)(q\cdot s_1\cdot u_2)q^2\\
&-2(k\cdot q)(k\cdot u_1)(k\cdot u_2)(q\cdot s_1\cdot u_2)-2(k\cdot u_1)(k\cdot u_2)^2(k\cdot s_1\cdot q)-\gamma(k\cdot q)(q\cdot s_1\cdot u_2)q^2-\gamma(k\cdot u_2)(k\cdot s_1\cdot q)q^2]{u_2}^{\mu}{u_2}^{\nu}\\
&-2\gamma(q\cdot s_1\cdot u_2)k^{\mu}q^{\nu}-\frac{q^2}{(k\cdot u_1)^2}[\gamma(k\cdot q)(k\cdot s_1\cdot u_2)+(k\cdot u_1)(k\cdot u_2)(k\cdot s_1\cdot u_2)-\gamma(k\cdot q)(q\cdot s_1\cdot u_2)\\
&-(k\cdot u_1)(k\cdot u_2)(q\cdot s_1\cdot u_2)]{u_1}^{\mu}{u_1}^{\nu}\Bigg]
\end{aligned}
$$

$t^{\mu\nu}_{s_2}$ Equal to $t^{\mu\nu}_{s_1}$ after interchanging the body labels $1\leftrightarrow 2$ and mapping $q\mapsto k-q$

$$
\begin{aligned}
t^{\mu\nu}_{s_1s_2}\quad &\mathrm{Sym}\Bigg[\frac{1}{2}[\gamma(k\cdot q)(q\cdot s_1\cdot s_2\cdot k)+\gamma(k\cdot s_1\cdot q)(k\cdot s_2\cdot q)+\gamma(q\cdot s_1\cdot s_2\cdot q)q^2+(k\cdot q)(q\cdot s_1\cdot u_2)(q\cdot s_2\cdot u_1)\\
&+(k\cdot u_1)(k\cdot u_2)(q\cdot s_1\cdot s_2\cdot k)+(k\cdot u_2)(k\cdot s_1\cdot q)(k\cdot s_2\cdot u_1)+(k\cdot s_2\cdot u_1)(q\cdot s_1\cdot u_2)q^2-\gamma(k\cdot q)(q\cdot s_1\cdot s_2\cdot q)\\
&-\gamma(q\cdot s_1\cdot s_2\cdot k)q^2-(k\cdot q)(k\cdot s_2\cdot u_1)(q\cdot s_1\cdot u_2)-(k\cdot u_1)(k\cdot u_2)(q\cdot s_1\cdot s_2\cdot q)-(k\cdot u_1)(k\cdot s_2\cdot q)(q\cdot s_1\cdot u_2)\\
&-(k\cdot u_2)(k\cdot s_1\cdot q)(q\cdot s_2\cdot u_1)-(q\cdot s_1\cdot u_2)(q\cdot s_2\cdot u_1)q^2]\eta^{\mu\nu}+[\gamma(q\cdot s_1\cdot s_2\cdot k)+(q\cdot s_1\cdot u_2)(q\cdot s_2\cdot u_1)-\gamma(q\cdot s_1\cdot s_2\cdot q)\\
&-(k\cdot s_2\cdot u_1)(q\cdot s_1\cdot u_2)]k^{\mu}k^{\nu}+[\gamma(q\cdot s_1\cdot s_2\cdot q)+(k\cdot s_2\cdot u_1)(q\cdot s_1\cdot u_2)-\gamma(q\cdot s_1\cdot s_2\cdot k)-(q\cdot s_1\cdot u_2)(q\cdot s_2\cdot u_1)]k^{\mu}q^{\nu}\\
&+\frac{q^2}{2(k\cdot u_1)}[2\gamma k^{\rho}(k\cdot s_2\cdot u_1)+(k\cdot u_1)(q\cdot s_2\cdot u_1){u_2}^{\rho}-2\gamma k^{\rho}(q\cdot s_2\cdot u_1)-(k\cdot u_1)(k\cdot s_2\cdot u_1){u_2}^{\rho}]k^{\mu}{s_1}^{\nu}{}_{\rho}\\
&+\frac{\gamma q^2}{2}(q^{\rho}-k^{\rho})k^{\mu}{s_1}^{\nu\sigma}{s_2}_{\rho\sigma}+[\gamma k^{\rho}(k\cdot s_1\cdot q)+q^{\rho}(k\cdot u_1)(q\cdot s_1\cdot u_2)-\gamma q^{\rho}(k\cdot s_1\cdot q)-k^{\rho}(k\cdot u_1)(q\cdot s_1\cdot u_2)]k^{\mu}{s_2}^{\nu}{}_{\rho}\\
&+\frac{q^2}{2(k\cdot u_1)}[2\gamma(q\cdot s_1\cdot s_2\cdot k)+2(q\cdot s_1\cdot u_2)(q\cdot s_2\cdot u_1)+\gamma(k\cdot s_1\cdot s_2\cdot q)+(k\cdot s_1\cdot u_2)(k\cdot s_2\cdot u_1)-2\gamma(q\cdot s_1\cdot s_2\cdot q)\\
&-2(k\cdot s_2\cdot u_1)(q\cdot s_1\cdot u_2)-\gamma(k\cdot s_1\cdot s_2\cdot k)-(k\cdot s_1\cdot u_2)(q\cdot s_2\cdot u_1)]k^{\mu}{u_1}^{\nu}+[(k\cdot u_1)(q\cdot s_1\cdot s_2\cdot q)+(k\cdot s_1\cdot q)(q\cdot s_2\cdot u_1)\\
&-(k\cdot u_1)(q\cdot s_1\cdot s_2\cdot k)-(k\cdot s_1\cdot q)(k\cdot s_2\cdot u_1)]k^{\mu}{u_2}^{\nu}+\frac{\gamma}{2}[2(k\cdot q)-q^2]q^{\mu}q^{\rho}{s_1}_{\rho}{}^{\sigma}{s_2}^{\nu}{}_{\sigma}\\
&+\frac{(k\cdot u_2)}{2}[q^2-2(k\cdot q)]q^{\rho}{s_1}_{\rho}{}^{\sigma}{s_2}^{\mu}{}_{\sigma}{u_1}^{\nu}+[\gamma(q\cdot s_1\cdot s_2\cdot k)+(q\cdot s_1\cdot u_2)(q\cdot s_2\cdot u_1)-\gamma(q\cdot s_1\cdot s_2\cdot q)\\
&-(k\cdot s_2\cdot u_1)(q\cdot s_1\cdot u_2)]q^{\mu}q^{\nu}+\frac{1}{2(k\cdot u_1)}[2\gamma k^{\rho}(q\cdot s_2\cdot u_1)q^2+2q^{\rho}(k\cdot u_1)(k\cdot u_2)(q\cdot s_2\cdot u_1)+(k\cdot u_1)(k\cdot s_2\cdot u_1)q^2{u_2}^{\rho}\\
&-2\gamma k^{\rho}(k\cdot s_2\cdot u_1)q^2-2\gamma q^{\rho}(k\cdot u_1)(k\cdot s_2\cdot q)-2q^{\rho}(k\cdot u_1)(k\cdot u_2)(k\cdot s_2\cdot u_1)-(k\cdot u_1)(q\cdot s_2\cdot u_1)q^2{u_2}^{\rho}]q^{\mu}{s_1}^{\nu}{}_{\rho}\\
&+\frac{\gamma q^2}{2}(k^{\rho}-q^{\rho})q^{\mu}{s_1}^{\nu\sigma}{s_2}_{\rho\sigma}+\frac{1}{2(k\cdot u_2)}[2\gamma k^{\rho}(q\cdot s_1\cdot u_2)q^2+2\gamma q^{\rho}(k\cdot u_2)(k\cdot s_1\cdot q)+2k^{\rho}(k\cdot u_1)(k\cdot u_2)(q\cdot s_1\cdot u_2)\\
&+2(k\cdot q)(k\cdot u_2)(q\cdot s_1\cdot u_2){u_1}^{\rho}-2\gamma k^{\rho}(k\cdot u_2)(k\cdot s_1\cdot q)-2q^{\rho}(k\cdot u_1)(k\cdot u_2)(q\cdot s_1\cdot u_2)-4\gamma k^{\rho}(k\cdot q)(q\cdot s_1\cdot u_2)\\
&-(k\cdot u_2)(q\cdot s_1\cdot u_2)q^2{u_1}^{\rho}]q^{\mu}{s_2}^{\nu}{}_{\rho}+\frac{1}{2(k\cdot u_1)}[2\gamma(q\cdot s_1\cdot s_2\cdot q)q^2+2(k\cdot u_1)(k\cdot u_2)(q\cdot s_1\cdot s_2\cdot q)\\
&+2(k\cdot u_1)(k\cdot s_2\cdot q)(q\cdot s_1\cdot u_2)+2(k\cdot s_2\cdot u_1)(q\cdot s_1\cdot u_2)q^2+\gamma(k\cdot s_1\cdot s_2\cdot k)q^2+(k\cdot s_1\cdot u_2)(q\cdot s_2\cdot u_1)q^2\\
&-2\gamma(q\cdot s_1\cdot s_2\cdot k)q^2-2(k\cdot u_1)(k\cdot u_2)(q\cdot s_1\cdot s_2\cdot k)-2(q\cdot s_1\cdot u_2)(q\cdot s_2\cdot u_1)q^2-\gamma(k\cdot s_1\cdot s_2\cdot q)q^2\\
&-(k\cdot s_1\cdot u_2)(k\cdot s_2\cdot u_1)q^2]q^{\mu}{u_1}^{\nu}+\frac{1}{2(k\cdot u_2)}[2(k\cdot q)(k\cdot s_2\cdot u_1)(q\cdot s_1\cdot u_2)+2(k\cdot u_1)(k\cdot u_2)(q\cdot s_1\cdot s_2\cdot k)\\
&+2(k\cdot u_2)(k\cdot s_1\cdot q)(k\cdot s_2\cdot u_1)+2(q\cdot s_1\cdot u_2)(q\cdot s_2\cdot u_1)q^2+4\gamma(k\cdot q)(q\cdot s_1\cdot s_2\cdot q)+\gamma(q\cdot s_1\cdot s_2\cdot k)q^2\\
&-2\gamma(k\cdot q)(q\cdot s_1\cdot s_2\cdot k)-2\gamma(q\cdot s_1\cdot s_2\cdot q)q^2-2(k\cdot u_1)(k\cdot u_2)(q\cdot s_1\cdot s_2\cdot q)-2(k\cdot u_2)(k\cdot s_1\cdot q)(q\cdot s_2\cdot u_1)\\
&-4(k\cdot q)(q\cdot s_1\cdot u_2)(q\cdot s_2\cdot u_1)-(k\cdot s_2\cdot u_1)(q\cdot s_1\cdot u_2)q^2]q^{\mu}{u_2}^{\nu}+\frac{1}{2}[2q^{\rho}(k\cdot q)(k\cdot u_2){u_1}^{\sigma}+\gamma k^{\rho}k^{\sigma}q^2-2q^{\rho}q^{\sigma}(k\cdot u_1)(k\cdot u_2)\\
&-\gamma k^{\rho}q^{\sigma}q^2-q^{\rho}(k\cdot u_2)q^2{u_1}^{\sigma}]{s_1}^{\mu}{}_{\rho}{s_2}^{\nu}{}_{\sigma}+\frac{1}{2(k\cdot u_1)^2}[2\gamma k^{\rho}(k\cdot q)(k\cdot s_2\cdot u_1)q^2+4q^{\rho}(k\cdot u_1)^2(k\cdot u_2)(k\cdot s_2\cdot q)
\end{aligned}
$$

$$+ \gamma k^\rho (k\cdot u_1)(k\cdot s_2\cdot q)q^2 + \gamma q^\rho (k\cdot u_1)(k\cdot s_2\cdot q)q^2 + k^\rho (k\cdot u_1)(k\cdot u_2)(k\cdot s_2\cdot u_1)q^2 + (k\cdot q)(k\cdot u_1)(q\cdot s_2\cdot u_1)q^2 u_2{}^\rho$$

$$+ q^\rho (k\cdot u_1)(k\cdot u_2)(k\cdot s_2\cdot u_1)q^2 - 2\gamma k^\rho (k\cdot q)(q\cdot s_2\cdot u_1)q^2 - k^\rho (k\cdot u_1)(k\cdot u_2)(q\cdot s_2\cdot u_1)q^2 - (k\cdot q)(k\cdot u_1)(k\cdot s_2\cdot u_1)q^2 u_2{}^\rho$$

$$- (k\cdot u_1)^2(k\cdot s_2\cdot q)q^2 u_2{}^\rho - q^\rho (k\cdot u_1)(k\cdot u_2)(q\cdot s_2\cdot u_1)q^2] s_1{}^\mu{}_\rho u_1{}^\nu + \frac{1}{2(k\cdot u_2)}[2\gamma q^\rho (k\cdot q)(k\cdot s_2\cdot q)$$

$$+ k^\rho (k\cdot u_2)(q\cdot s_2\cdot u_1)q^2 + q^\rho (k\cdot u_2)(q\cdot s_2\cdot u_1)q^2 - 2q^\rho (k\cdot q)(k\cdot u_2)(q\cdot s_2\cdot u_1) - 2q^\rho (k\cdot u_1)(k\cdot u_2)(k\cdot s_2\cdot q)$$

$$- \gamma q^\rho (k\cdot s_2\cdot q)q^2 - k^\rho (k\cdot u_2)(k\cdot s_2\cdot u_1)q^2] s_1{}^\mu{}_\rho u_2{}^\nu + \frac{(k\cdot u_1)q^2}{2}(k^\rho - q^\rho) s_1{}^{\mu\sigma} s_{2\,\rho\sigma} u_2{}^\nu + \frac{1}{2}[2k^\rho q^\sigma (k\cdot u_1)(k\cdot u_2) + \gamma k^\rho q^\sigma q^2$$

$$+ q^\rho (k\cdot u_1)q^2 u_2{}^\sigma - 2\gamma k^\rho q^\sigma (k\cdot q) - k^\rho (k\cdot u_1)q^2 u_2{}^\sigma] s_1{}^\mu{}_\sigma s_2{}^\nu{}_\rho + \frac{1}{2(k\cdot u_1)}[2k^\rho (k\cdot q)(k\cdot u_1)(q\cdot s_1\cdot u_2)$$

$$+ 2k^\rho (k\cdot u_1)(k\cdot u_2)(k\cdot s_1\cdot q) + \gamma k^\rho (k\cdot s_1\cdot q)q^2 + k^\rho (k\cdot u_1)(k\cdot s_1\cdot u_2)q^2 + q^\rho (k\cdot u_1)(q\cdot s_1\cdot u_2)q^2$$

$$- 2k^\rho (k\cdot u_1)(q\cdot s_1\cdot u_2)q^2 - 2q^\rho (k\cdot u_1)(k\cdot u_2)(k\cdot s_1\cdot q) - \gamma q^\rho (k\cdot s_1\cdot q)q^2 - q^\rho (k\cdot u_1)(k\cdot s_1\cdot u_2)q^2] s_2{}^\mu{}_\rho u_1{}^\nu$$

$$+ \frac{1}{2(k\cdot u_2)^2}[2k^\rho (k\cdot u_1)(k\cdot u_2)(q\cdot s_1\cdot u_2)q^2 + 2q^\rho (k\cdot q)(k\cdot u_1)(k\cdot u_2)(q\cdot s_1\cdot u_2) + 4\gamma k^\rho (k\cdot q)^2(q\cdot s_1\cdot u_2)$$

$$+ 4\gamma k^\rho (k\cdot q)(k\cdot u_2)(k\cdot s_1\cdot q) + 4q^\rho (k\cdot u_1)(k\cdot u_2)^2(k\cdot s_1\cdot q) + \gamma q^\rho (k\cdot u_2)(k\cdot s_1\cdot q)q^2 + (k\cdot q)(k\cdot u_2)(q\cdot s_1\cdot u_2)q^2 u_1{}^\rho$$

$$+ (k\cdot u_2)^2(k\cdot s_1\cdot q)q^2 u_1{}^\rho - 2\gamma k^\rho (k\cdot q)(q\cdot s_1\cdot u_2)q^2 - 2\gamma k^\rho (k\cdot u_2)(k\cdot s_1\cdot q)q^2 - 2\gamma q^\rho (k\cdot q)(k\cdot u_2)(k\cdot s_1\cdot q)$$

$$- 2(k\cdot q)^2(k\cdot u_2)(q\cdot s_1\cdot u_2)u_1{}^\rho - 2(k\cdot q)(k\cdot u_2)^2(k\cdot s_1\cdot q)u_1{}^\rho - 4k^\rho (k\cdot q)(k\cdot u_1)(k\cdot u_2)(q\cdot s_1\cdot u_2)$$

$$- 4k^\rho (k\cdot u_1)(k\cdot u_2)^2(k\cdot s_1\cdot q) - q^\rho (k\cdot u_1)(k\cdot u_2)(q\cdot s_1\cdot u_2)q^2] s_2{}^\mu{}_\rho u_2{}^\nu + \frac{q^2}{2(k\cdot u_1)^2}[\gamma (k\cdot q)(k\cdot s_1\cdot s_2\cdot q)$$

$$+ \gamma (k\cdot q)(q\cdot s_1\cdot s_2\cdot k) + (k\cdot q)(k\cdot s_1\cdot u_2)(k\cdot s_2\cdot u_1) + (k\cdot q)(q\cdot s_1\cdot u_2)(q\cdot s_2\cdot u_1) + (k\cdot u_1)(k\cdot u_2)(k\cdot s_1\cdot s_2\cdot q)$$

$$+ (k\cdot u_1)(k\cdot u_2)(q\cdot s_1\cdot s_2\cdot k) + (k\cdot u_1)(k\cdot s_1\cdot u_2)(k\cdot s_2\cdot q) - \gamma (k\cdot q)(k\cdot s_1\cdot s_2\cdot k) - \gamma (k\cdot q)(q\cdot s_1\cdot s_2\cdot q)$$

$$- (k\cdot q)(k\cdot s_1\cdot u_2)(q\cdot s_2\cdot u_1) - (k\cdot q)(k\cdot s_2\cdot u_1)(q\cdot s_1\cdot u_2) - (k\cdot u_1)(k\cdot u_2)(k\cdot s_1\cdot s_2\cdot k) - (k\cdot u_1)(k\cdot u_2)(q\cdot s_1\cdot s_2\cdot q)$$

$$- (k\cdot u_1)(k\cdot s_2\cdot q)(q\cdot s_1\cdot u_2)] u_1{}^\mu u_1{}^\nu + \frac{1}{2(k\cdot u_1)(k\cdot u_2)}[2(k\cdot u_1)(k\cdot u_2)(q\cdot s_1\cdot s_2\cdot q)q^2 + (k\cdot u_1)(k\cdot u_2)(k\cdot s_1\cdot s_2\cdot k)q^2$$

$$+ (k\cdot u_1)(k\cdot s_2\cdot q)(q\cdot s_1\cdot u_2)q^2 + (k\cdot u_2)(k\cdot s_1\cdot q)(q\cdot s_2\cdot u_1)q^2 - 2(k\cdot q)(k\cdot u_1)(k\cdot u_2)(q\cdot s_1\cdot s_2\cdot q)$$

$$- 2(k\cdot q)(k\cdot u_1)(k\cdot s_2\cdot q)(q\cdot s_1\cdot u_2) - 2(k\cdot u_1)(k\cdot u_2)(k\cdot s_1\cdot q)(k\cdot s_2\cdot q) - (k\cdot u_1)(k\cdot u_2)(k\cdot s_1\cdot s_2\cdot q)q^2$$

$$- (k\cdot u_1)(k\cdot u_2)(q\cdot s_1\cdot s_2\cdot k)q^2 - (k\cdot u_2)(k\cdot s_1\cdot q)(k\cdot s_2\cdot u_1)q^2] u_1{}^\mu u_2{}^\nu + \frac{1}{2(k\cdot u_2)^2}[2(k\cdot q)^2(q\cdot s_1\cdot u_2)(q\cdot s_2\cdot u_1)$$

$$+ 2(k\cdot q)(k\cdot u_1)(k\cdot u_2)(q\cdot s_1\cdot s_2\cdot q) + 2(k\cdot q)(k\cdot u_2)(k\cdot s_1\cdot q)(q\cdot s_2\cdot u_1) + \gamma (k\cdot q)(q\cdot s_1\cdot s_2\cdot q)q^2$$

$$- 2\gamma (k\cdot q)^2(q\cdot s_1\cdot s_2\cdot q) - (k\cdot q)(q\cdot s_1\cdot u_2)(q\cdot s_2\cdot u_1)q^2 - (k\cdot u_1)(k\cdot u_2)(q\cdot s_1\cdot s_2\cdot q)q^2$$

$$- (k\cdot u_2)(k\cdot s_1\cdot q)(q\cdot s_2\cdot u_1)q^2] u_2{}^\mu u_2{}^\nu - \frac{1}{2(k\cdot u_2)}[2\gamma (k\cdot q)^2 + (k\cdot u_1)(k\cdot u_2)q^2 - 2(k\cdot q)(k\cdot u_1)(k\cdot u_2)$$

$$- \gamma (k\cdot q)q^2] q^\rho s_{1\,\rho}{}^\sigma s_2{}^\mu{}_\sigma u_2{}^\nu - \frac{q^2}{2(k\cdot u_1)}[\gamma k^\rho (k\cdot q) + k^\rho (k\cdot u_1)(k\cdot u_2) - \gamma q^\rho (k\cdot q) - q^\rho (k\cdot u_1)(k\cdot u_2)] s_1{}^{\mu\sigma} s_{2\,\rho\sigma} u_1{}^\nu \Big]$$

$t^{\mu\nu}_{s_1 s_1}$

$$\mathrm{Sym}\Big[ q^2[(k\cdot s_1\cdot u_2) - (q\cdot s_1\cdot u_2)] k^\rho s_1{}^\mu{}_\rho u_2{}^\nu + \frac{q^2}{d-2}(q^\sigma - k^\sigma)k^\rho s_1{}^\mu{}_\rho s_1{}^\nu{}_\sigma + \frac{\gamma q^2}{(k\cdot u_1)}[(q\cdot s_1\cdot u_2) - (k\cdot s_1\cdot u_2)] k^\mu k^\rho s_1{}^\nu{}_\rho$$

$$+ \frac{\gamma q^2}{(k\cdot u_1)}[(k\cdot s_1\cdot u_2) - (q\cdot s_1\cdot u_2)] k^\rho q^\mu s_1{}^\nu{}_\rho - \frac{q^2}{(d-2)(k\cdot u_1)^2}[(d-2)(k\cdot u_1)(k\cdot u_2)(k\cdot s_1\cdot u_2) + \gamma (d-2)(k\cdot q)(k\cdot s_1\cdot u_2)$$

$$+ (k\cdot u_1)(k\cdot s_1\cdot q) - (d-2)(k\cdot u_1)(k\cdot u_2)(q\cdot s_1\cdot u_2) - \gamma (d-2)(k\cdot q)(q\cdot s_1\cdot u_2)] k^\rho s_1{}^\mu{}_\rho u_1{}^\nu + \beta_\gamma C_{E_1}(q\cdot s_1\cdot s_1\cdot q)k^\mu q^\nu$$

$$+ C_{E_1} q^2[\beta_\gamma q^\rho + \gamma (k\cdot u_1)u_2{}^\rho - \beta_\gamma k^\rho] k^\mu s_1{}^{\nu\sigma} s_{1\,\rho\sigma} + C_{E_1} q^2[\beta_\gamma k^\rho - \beta_\gamma q^\rho - \gamma (k\cdot u_1)u_2{}^\rho] q^\mu s_1{}^{\nu\sigma} s_{1\,\rho\sigma} + C_{E_1}[2\gamma (q\cdot s_1\cdot s_1\cdot q)q^2$$

$$+ 2(k\cdot u_1)(k\cdot u_2)(q\cdot s_1\cdot s_1\cdot q) + \gamma (k\cdot s_1\cdot s_1\cdot k)q^2 - 2\gamma (k\cdot q)(q\cdot s_1\cdot s_1\cdot q) - \gamma (k\cdot s_1\cdot s_1\cdot q)q^2$$

$$- (k\cdot u_1)(k\cdot s_1\cdot s_1\cdot u_2)q^2] u_1{}^\mu u_2{}^\nu - \beta_\gamma C_{E_1}(q\cdot s_1\cdot s_1\cdot q)k^\mu k^\nu - \beta_\gamma C_{E_1}(q\cdot s_1\cdot s_1\cdot q)q^\mu q^\nu - C_{E_1}(k\cdot u_1)q^2[\gamma q^\rho + (k\cdot u_1)u_2{}^\rho$$

$$- \gamma k^\rho] s_1{}^{\mu\sigma} s_{1\,\rho\sigma} u_2{}^\nu + \frac{2C_{E_1}(q\cdot s_1\cdot s_1\cdot q)}{d-2}[\gamma (d-2)(k\cdot u_1) + (k\cdot u_2)] k^\mu u_2{}^\nu - \frac{C_{E_1}(k\cdot u_1)^2 q^2}{d-2} s_1{}^{\mu\rho} s_1{}^\nu{}_\rho$$

$$
\begin{aligned}
&-\frac{C_{E_1}(q\cdot s_1\cdot s_1\cdot q)}{2(d-2)}[2\gamma(d-2)(k\cdot u_1)(k\cdot u_2)+2(k\cdot u_1)^2+2(k\cdot u_2)^2+\beta_\gamma(d-2)(k\cdot q)-\beta_\gamma(d-2)q^2]\eta^{\mu\nu}\\
&+\frac{C_{E_1}}{(k\cdot u_1)}[2\gamma(k\cdot u_1)(k\cdot u_2)(q\cdot s_1\cdot s_1\cdot q)+\beta_\gamma(k\cdot s_1\cdot s_1\cdot k)q^2+\beta_\gamma(q\cdot s_1\cdot s_1\cdot q)q^2-\beta_\gamma(k\cdot s_1\cdot s_1\cdot q)q^2\\
&-\gamma(k\cdot u_1)(k\cdot s_1\cdot s_1\cdot u_2)q^2]q^\mu u_1{}^\nu+\frac{C_{E_1}}{(d-2)(k\cdot u_1)}[2(k\cdot u_1)^2(q\cdot s_1\cdot s_1\cdot q)+\beta_\gamma(d-2)(k\cdot s_1\cdot s_1\cdot q)q^2\\
&+\gamma(d-2)(k\cdot u_1)(k\cdot s_1\cdot s_1\cdot u_2)q^2-\beta_\gamma(d-2)(k\cdot s_1\cdot s_1\cdot k)q^2-\beta_\gamma(d-2)(q\cdot s_1\cdot s_1\cdot q)q^2]k^\mu u_1{}^\nu\\
&+\frac{C_{E_1}q^2}{(d-2)(k\cdot u_1)}[2k^\rho(k\cdot u_1)^2+\beta_\gamma(d-2)q^\rho(k\cdot q)+(d-2)(k\cdot u_1)^2(k\cdot u_2)u_2{}^\rho+\gamma(d-2)(k\cdot q)(k\cdot u_1)u_2{}^\rho\\
&+\gamma(d-2)q^\rho(k\cdot u_1)(k\cdot u_2)-\beta_\gamma(d-2)k^\rho(k\cdot q)-\gamma(d-2)k^\rho(k\cdot u_1)(k\cdot u_2)]s_1{}^{\mu\sigma}s_{1\,\rho\sigma}u_1{}^\nu\\
&+\frac{C_{E_1}}{2(d-2)(k\cdot u_1)^2}[2\beta_\gamma(d-2)(k\cdot q)(k\cdot s_1\cdot s_1\cdot q)q^2+2(d-2)(k\cdot u_1)^2(k\cdot u_2)(k\cdot s_1\cdot s_1\cdot u_2)q^2\\
&+2\gamma(d-2)(k\cdot q)(k\cdot u_1)(k\cdot s_1\cdot s_1\cdot u_2)q^2+2\gamma(d-2)(k\cdot u_1)(k\cdot u_2)(k\cdot s_1\cdot s_1\cdot q)q^2+2(k\cdot u_1)^2(k\cdot s_1\cdot s_1\cdot k)q^2\\
&-2\beta_\gamma(d-2)(k\cdot q)(k\cdot s_1\cdot s_1\cdot k)q^2-2(d-2)(k\cdot u_1)^2(k\cdot u_2)^2(q\cdot s_1\cdot s_1\cdot q)-2\gamma(d-2)(k\cdot u_1)(k\cdot u_2)(k\cdot s_1\cdot s_1\cdot k)q^2\\
&-2\gamma(d-2)(k\cdot u_1)(k\cdot u_2)(q\cdot s_1\cdot s_1\cdot q)q^2-\beta_\gamma(d-2)(k\cdot q)(q\cdot s_1\cdot s_1\cdot q)q^2]u_1{}^\mu u_1{}^\nu+\frac{C_{E_1}(q\cdot s_1\cdot s_1\cdot q)}{(k\cdot u_2)}[2\beta_\gamma(k\cdot q)\\
&-2\gamma(k\cdot u_1)(k\cdot u_2)-\beta_\gamma q^2]q^\mu u_2{}^\nu+\frac{C_{E_1}(q\cdot s_1\cdot s_1\cdot q)}{2(k\cdot u_2)^2}[4\gamma(k\cdot q)(k\cdot u_1)(k\cdot u_2)+\beta_\gamma(k\cdot q)q^2-2\beta_\gamma(k\cdot q)^2\\
&-2\gamma(k\cdot u_1)(k\cdot u_2)q^2-2(k\cdot u_1)^2(k\cdot u_2)^2]u_2{}^\mu u_2{}^\nu\Big]
\end{aligned}
$$

$t^{\mu\nu}_{s_2 s_2}$ Equal to $t^{\mu\nu}_{s_1 s_1}$ after interchanging the body labels $1 \leftrightarrow 2$ and mapping $q \mapsto k-q$
